# Supplementary material for: Visualizing the Diversity of Representations Learned by Bayesian Neural Networks
Source: arXiv:2201.10859 source file (2023-11-14)
Supplement: Supplementary file 1 [file appendix_ms_cifar100_fvs.pdf]

## WRes0.7

Cluster 1

Cluster 2

Cluster 3

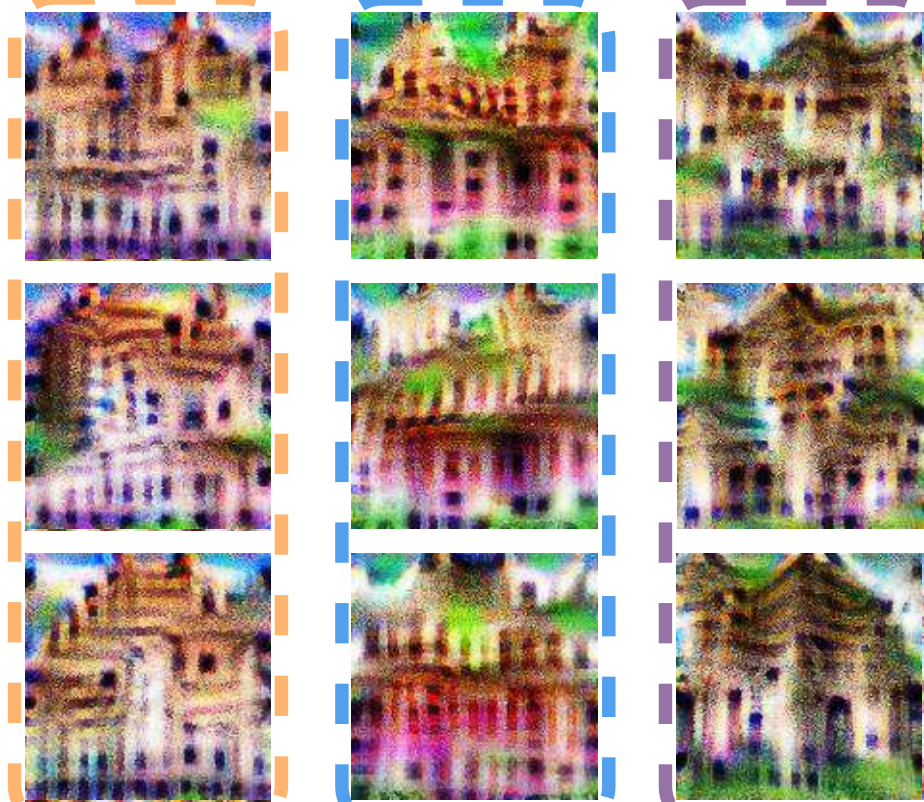

tSNE component 2

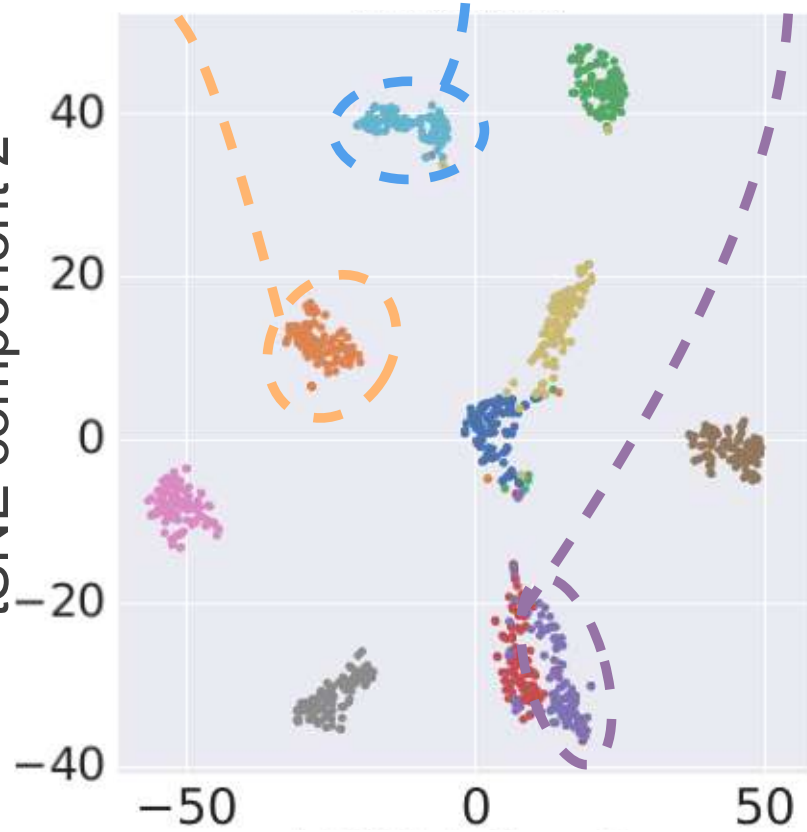

tSNE component 1

## WRes2

Cluster 1

Cluster 2

Cluster 3

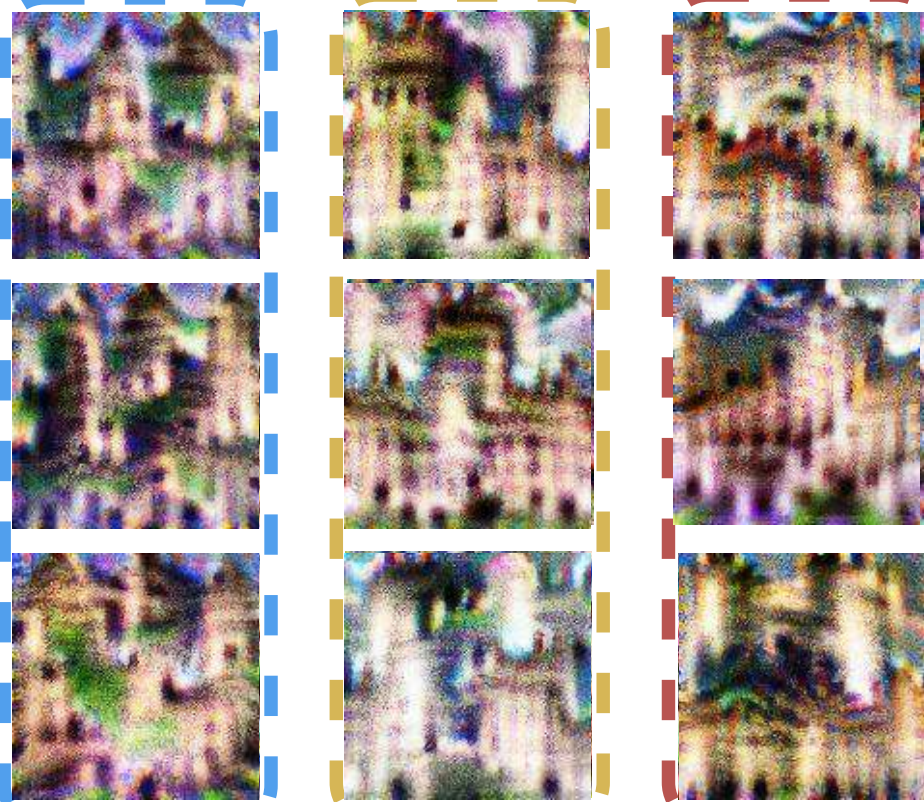

tSNE component 2

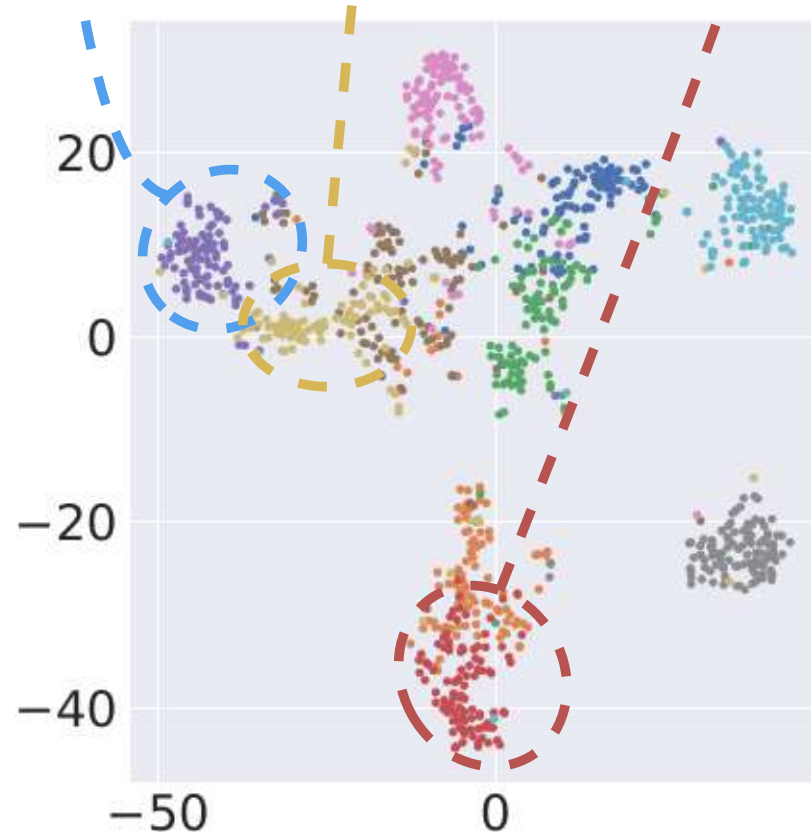

tSNE component 1
